# Supplementary material for: VSRD: Instance-Aware Volumetric Silhouette Rendering for Weakly Supervised 3D Object Detection
Source: arXiv:2404.00149 source file (2024-03-29)
Supplement: Supplementary file 2 [file main.tex]

\subsubsection{Semi-Supervised Setting}
\label{sec:additional_visualization_results/monocular_3d_object_detection/semi_supervised_setting}

We show additional visualization results of semi-supervised monocular 3D object detection in \cref{fig:additional_visualization_results/monocular_3d_object_detection/semi_supervised_setting/monodetr} and \cref{fig:additional_visualization_results/monocular_3d_object_detection/semi_supervised_setting/monoflex}, comparing our method with MonoDETR \cite{MonoDETR} and MonoFlex \cite{MonoFlex}, respectively. The detectors fine-tuned on a subset of the whole data demonstrate enhanced performance, surpassing those trained on the whole data from scratch.
