# Supplementary material for: VSRD: Instance-Aware Volumetric Silhouette Rendering for Weakly Supervised 3D Object Detection
Source: arXiv:2404.00149 source file (2024-03-29)
Supplement: Supplementary file 3 [file main.tex]

\subsubsection{Weakly Supervised Setting}
\label{sec:additional_visualization_results/monocular_3d_object_detection/weakly_supervised_setting}

Additional visualization results of weakly supervised monocular 3D object detection can be seen in \cref{fig:additional_visualization_results/monocular_3d_object_detection/weakly_supervised_setting}. Compared with WeakM3D \cite{WeakM3D} and Autolabels \cite{Autolabels}, our method demonstrates superior performance in both perspective and bird's eye views. WeakM3D struggles to estimate the orientations of laterally moving objects accurately because it assumes that most cars are forward-facing, resulting in suboptimal estimation for laterally moving objects. In contrast, our method leverages pseudo labels generated by the proposed auto-labeling for 3D supervision without fixed priors, leading to more accurate orientation estimation. Furthermore, for the comparison with Autolabels, which faces challenges in accurately estimating 3D bounding boxes, particularly in their vertical locations, our method demonstrates superior 
performance, affirming the high quality of our pseudo labels.
