# Supplementary material for: VSRD: Instance-Aware Volumetric Silhouette Rendering for Weakly Supervised 3D Object Detection
Source: arXiv:2404.00149 source file (2024-03-29)
Supplement: Supplementary file 4 [file main.tex]

\subsection{Multi-View 3D Auto-Labeling}
We show more visualization results of the 3D bounding boxes optimized by our proposed multi-view 3D auto-labeling. As shown in \cref{fig:additional_visualization_results/multi_view_3d_auto_labeling}, it is evident that our proposed multi-view 3D auto-labeling demonstrates proficiency in accurately reconstructing instance surfaces, even in the presence of occlusions. For instance, for the occluded pink vehicle showcased in the second column, despite the challenge of occlusion, our approach effectively renders the surface details and optimizes the 3D bounding box, which verifies the strength of our proposed instance-aware volumetric rendering when dealing with scenes with complex geometric relationships among instances, such as occlusions.
